# Supplementary material for: Adaptation of the Independent Metropolis-Hastings Sampler with Normalizing Flow Proposals
Source: arXiv:2110.13216 source file (2021-10-25)
Supplement: Supplementary file 9 [file proofs-concerning-containment.tex]

\clearpage
\section{Proofs Concerning Containment}\label{app:proofs-concerning-containment}

\begin{proof}[Proof of \Cref{prop:containment-log-density}]
  \begin{align}
      & \mathrm{Pr}\left[\log \pi(x) - \log\tilde{\pi}_{\Theta_n}(x) < \log M~~\forall~~x\in\mathcal{X}\right] \geq 1-\delta~~\forall~~n\in\mathbb{N} \\
      \implies &\mathrm{Pr}\left[\frac{\pi(x)}{\tilde{\pi}_{\Theta_n}(x)} <  M~~\forall~~x\in\mathcal{X}\right] \geq 1-\delta~~\forall~~n\in\mathbb{N}
  \end{align}
  Then for all $\epsilon > 0$ there exists $N\equiv N(\epsilon, \delta)\in\mathbb{N}$ such that for all $x\in\mathcal{X}$,
  \begin{align}
      &\mathrm{Pr}\left[\Vert K_{\Theta_n}^N(x,\cdot) - \Pi(\cdot)\Vert_{\mathrm{TV}} <\epsilon\right]\geq 1-\delta ~~\forall~~n\in\mathbb{N}\\
      \implies& \mathrm{Pr}\left[W_\epsilon(x, K_{\Theta_n}) \leq N\right] \geq 1-\delta ~~\forall~~n\in\mathbb{N}.
  \end{align}
\end{proof}
